# Supplementary material for: DramatVis Personae: Visual Text Analytics for Identifying Social Biases in Creative Writing
Source: arXiv:2209.00320 source file (2022-09-01)
Supplement: Supplementary file 1 [file A_Kiss_of_Ice.pdf]

## Demographics

| Character       | Sex    | Ethnicity                           | Age                |
|-----------------|--------|-------------------------------------|--------------------|
| Richard Barnaby | Male   | White (American)                    | Middle-aged        |
| Christa Barnaby | Female | White (American)                    | Middle-aged        |
| Irina           | Female | White (Russian);<br>Demon; Succubus | Young (presenting) |
| Uwe Schmidt     | Male   | White (German)                      | Middle-aged        |
| Mr. Lee         | Male   | Asian (Singapore)                   | Old                |

## A Kiss of Ice

*Just one more run*, Richard Barnaby said to himself as he crested the last ridge, the big ski lodge and lift complex at the bottom of the slope looming out of the mist. He was cold and his legs were burning, but this was his last day in Valle d'Aosta and he was damned if he wasn't going to get the most out of it. He slid to a stop and turned around to look back upslope, plastering a big smile on his face that he hoped was not too obviously fake. He was pretty sure he knew how this was going to go.

Christa was far behind, of course, and she was taking her sweet time, as usual. He suppressed an exasperated sigh and leaned on his poles instead, his smile becoming even more strained.

"Looking good, hun," he remarked with forced joviality as she finally slid to a stop next to him, a sulky look on her face. "What do you say, one more run? Last chance!"

Christa wasn't having any of it. "I'm cold, honey," she said in that almost-whiny voice he had come to resent, her grimace turning into a full-blown pout. "I want to go back to the hotel."

"Aww, come on," he smiled, jabbing lightly at her with an elbow.

She pushed him away and scowled. "I said I'm cold," she countered. "Besides, didn't you tell me that you aren't supposed to call your last run?"

He chuckled, his smile finally becoming genuine. "You got me there. So two more runs, and skip the last?"

Not even a smile in response. "You go if you really have to," she said petulantly. "I'll be at the bar."

*I already knew that*, he thought to himself but didn't say. Instead he shrugged and smiled again. "Fine, but it'd be a lot more fun if you came too."

She had already turned her back and was poling away in the direction of the lodge and the glowing lights of the village beyond. "Remember, the live music starts at seven," she called over her shoulder. "I'll save you a space at the bar."

He sighed in resignation, looking at her retreating back for a moment, and then turned deftly on his skis and took off in the direction of the lift. It was getting late, he realized, almost five o'clock and closing time. The sun had plunged below the horizon and the slopes were already darkening visibly, the light snow mist filling the frigid air on a thousand hissing feet. He would have to hurry if he was going to catch the last gondola up the mountain. The crowd had thinned out, and the resort crew were bustling around in the half-light with their closing chores. Maybe he was already too late?

But when he rounded the corner of the lift complex, the huge wheel humming contentedly in the gloom inside the massive metal housing, he was gratified to see a small group of people unhurriedly poling ahead of him towards the lift entrance. Not too late then. He caught up to them, two men and a woman, and slid in behind. The line was deserted, with no lift crew in sight, and his heart sank again. Maybe they had closed down the lift after all? It was still running, but they may just be ferrying the last skiers up the slope.

But then the woman in the lead, clad in a bright white ski suit, reached the turnstile and went through with no trouble at all. Not locked then. Richard smiled in satisfaction, filing in through the turnstile after the two men. He would get a last run after all! Or, he corrected himself, two more runs, but he'd skip the second. He stepped out of his skis and lined up with the little group as they trod up the entrance ramp. The woman in white was just in front of him, and he couldn't resist sneaking a glance at her figure as he stepped up behind her. She was young and slim, and her tight snowsuit left little to the imagination.

The next gondola arrived, automatically slowing down in front of the ramp with its door already open to let them in. *Weird*, Richard thought to himself. *Normally there's someone here to make sure you get on all right.* He mentally shrugged. It was the end of the day, after all, and the temperature was dropping rapidly. He guessed he couldn't blame the staff for getting indoors to warm up. Besides, the lift was all automated. He was next in line to get aboard, so he shuffled up to the gap as the woman in white stepped in. That meant he saw her drop her pole almost before it happened, so he was able to reach out and catch it before it slipped between the gondola car and the ramp.

"Sorry, miss," he said, stepping into the gondola behind her and lightly putting a hand on her shoulder. "You dropped one of your ski poles."

"Oh," she exclaimed, turning around so abruptly that he almost dropped the pole he was proffering to her. Then she raised her gaze, and he almost dropped it again. Her face was heart-shaped and lovely, pale but framed by dark locks and with flushed cheeks the very picture of health. Still, it was her arrestingly large eyes that instantly captured his attention. They looked

almost purple in the ruddy glow of the gondola's interior. "Thank you so much, sir." Her English was heavily but charmingly accented. Russian, maybe?

The door of the gondola sighed shut behind him, and the car jerked gently as it started to gain speed. "It almost fell under the platform," he stammered, brandishing the pole and feeling the color in his face rise. Blushing? He hadn't blushed since high school three decades ago! He hoped it wouldn't be visible in the cabin's dim light.

She took it, smiling sweetly at him, and he felt his heart skip a beat. That smile was not very innocent at all, he realized, almost like she was laughing at him behind it. "Very kind," she said. She turned away to find a seat, and his heart sank at the loss.

He mentally shook himself and turned around to find his own seat. The gondola car was made for eight people, so with only four of them, there was plenty of space. Richard leaned his skis on the bright red wall next to the glass window, absently brushing snow off the bindings as he covertly looked over the other passengers. The woman was ignoring him, half turned away and gazing behind her towards the rapidly receding valley floor with her dark curls silhouetted against the glow of the village below. The two men were seated across from him, their heads together and engaged in deep conversation. One was tall and powerfully built, clad in a bright orange ski suit, and with a heavy beard rimed with frost. The other one was thin and short with a black jacket and white snow pants and a jaunty yellow beanie perched on his head. The latter man noticed Richard's attention, and as he turned his face to nod in recognition, Richard saw that he had Asian features. Richard nodded back and then averted his gaze, uncomfortable at getting caught ogling his co-passengers.

Out of the corner of his eye he saw the bearded man pull out a large black object from his breast pocket and show it to his partner. What was that? It almost looked like one of those new mobile phones that fit into your pocket, and he suddenly felt consumed by curiosity but unable to look back at the pair. He had already been caught staring once and he didn't feel particularly inclined to be caught again. But a mobile phone, here, in the Italian Alps? The bearded man said something and slipped the large object back into his breast pocket, and Richard quickly lost interest and directed his attention to the scenery gliding by beneath the gondola as it steadily ascended the mountain.

The snow was picking up, he noticed, just on schedule. The weather report in the hotel's lobby that morning had warned about an impending storm that would start to make itself known in the evening. Ten inches of snow was scheduled to fall overnight, maybe more, and Richard felt the first stirring of unease as he gazed out at the intensifying snowfall. He was a strong skier, but it was late, he was tired, and the darkness combined with the snow would make getting down the slope quite a challenge. Were the slopes even going to be passable with all this new snow? But then he spotted two cones of bright light cutting through the mist far below him. Good. A snow grooming machine was puffing its way down the mountain, so the resort crew were still working on getting the slopes ready for the next day. That hopefully meant he should be okay getting down on his own.

He lost himself to daydreaming for a while, the relative warmth and gentle rocking of the gondola having an oddly soothing effect on his tired body and mind. It was perhaps ten minutes later when the woman in white said something loudly in Italian that he looked up with a start. Her voice was clearly worried and she was looking out the window. She had spoken in Italian, so maybe she wasn't Russian after all?

She looked back at Richard, quickly meeting his gaze, and then at the other two men, who both looked back in confusion. "Why are we stopping, please?" she said in her accented English, clearly having repeated her initial statement when no one answered in kind.

She was right, he realized. The subtle hum of the cable car had changed, shifting down from a pleasant whine at the edge of hearing to a more low-pitched rumble. As he watched, a lift pylon materialized out of the gloom and then passed by the gondola's window. The lift was definitely slowing down.

"You're right," he said automatically, twisting to look out the window at the receding pylon, a claw of metal half already obscured by swirling clouds of snow. Visibility was down to fifty feet, he realized, and the rising storm was buffeting the car and whistling subtly through the worn rubber gasket around the accordion doors. As he moved away from the chill draft and watched, the car slowed further and came to a stop, rocking gently. All sound died away save for the quiet whine of the gathering wind. And then the light dome in the middle of the ceiling abruptly clicked off, plunging the cabin into the curious silvery darkness of a snowy midwinter night. Now the car was lit only by the harsh cold light of a fluorescent light fixture mounted on the nearby lift pylon, long shadows stretching across the cabin floor.

The bearded man cursed loudly in German. He was on his feet and thumped rapidly over to the door next to Richard to look out with his heavy ski boots, his rapid movement setting the gondola swinging from side to side. Richard felt his stomach lurch and instinctively grabbed the metal railing as he fell back into his seat. "*Scheiße*, they can't turn it off, we're still on the lift!" the man yelled to no one in particular, this time in clipped English.

His Asian partner was still seated, turning a mild face on the bearded man straining to look out the window into the thick swirls of snow. "Calm down, Uwe, this is just a misunderstanding," he said calmly in perfect English. "Have a seat and let's just wait until they turn the lift back on."

Richard nodded, but felt his heart racing. The man's abrupt charge at the door had been unexpected and terrifying. "Yes, sit down, please," he said. "There's nothing to be gained by panicking. I'm sure the lift will get going again in a minute."

Uwe turned to glare down at him in the half-light, white teeth gritted in his dark beard. "I'm not panicking, *mein Herr*," he said, but Richard thought he heard a quaver in the gruff voice. "Don't tell me what to do."

Richard swallowed, feeling the heat of the man's glare and the weight of his sheer physical presence. The gondola car was listing to one side because of the weight imbalance, and he felt himself idly wondering about the tensile strength of the cabin's steel frame in subzero temperatures. Surely it must have been built for precisely this kind of thing?

"Sure," he said meekly, inadvertently leaning back in his seat. "Just take it easy. I didn't mean anything by it."

"Take it easy?" the big man replied, the white grin turning decidedly feral. "*Scheiße*, I'm taking it easy. You don't want to see me not take it easy."

Richard swallowed again, desperately wondering how he had gotten himself into hot water so quickly. He wasn't sure what to say to de-escalate the situation, but then a gentle voice broke in from just behind the big German. "Sir, please," said the woman in white. She was standing very close, and when the man whirled around to face her, she placed her hand lightly on his chest inside his unzipped ski jacket. Despite the gloom in the cabin, Richard had a perfect view of the man's face relaxing almost instantly. Richard glanced at the girl—no, young woman, he corrected himself—and felt a stab of jealousy in his chest. Her big dark eyes were focused on the man as if he was the only other person in the world and her slender hand with its long and delicate fingers was very white in the gray light of the cabin, seeming almost to caress the man's chest.

"I'm frightened, sir," she said, her eyes turning pleading as she gazed up at the big man. Something about that look scratched at Richard's subconscious, and again he had the feeling that she was—laughing? surely not?—on the inside. "Will you sit with me?"

Russian for sure, Richard thought to himself as he observed the two, feeling his own heart calm down in his chest. That impromptu confrontation with the big German had left him rattled. The woman did sound scared, but Richard wasn't sure she was really acting the part. Why did he get the distinct impression that this was just an act? Was she merely playing the damsel in distress card to defuse the situation?

As if in response to this thought, she glanced his way briefly, and he was struck speechless by the intense look in her dark purple eyes. She wasn't just beautiful, she was radiant in the muted silver darkness, the swirling snow outside giving the fluorescent light the illusion of dappled waves rippling across her face. High Slavic cheekbones, satin skin, and a too-sharp chin gave her an almost feline appearance. And those eyes. She didn't smile, but there was something... hungry in them. Then she looked back at Uwe the German, and he could breathe again.

Uwe wasn't noticing any of this. He stammered, deflating somewhat and turning beet red under the black beard. "*Natürlich, natürlich, fräulein*," he muttered, all the bravado gone in an instant. His hand rose to almost grasp hers, and then he seemed to think better of it and let it fall. "*Entschuldigung*... Of course I will sit with you."

Without hesitation, her hand did come down to clasp his, and she resolutely turned and guided him back to her seat, towing the man behind her like she was bringing a new partner to the dance floor. They sat down, and Richard noted that the woman snuggled up next to the man and placed a hand lightly on his big leg, as if in reassurance. The man turned big worshipful eyes on her to watch her every move.

The Asian man looked bemused, staring at his partner with a slight smile playing on his lips. "That's very well, Uwe," he said, casting a sharp glance at Richard in the half light. "If you're

done comforting the young miss, perhaps you can help do something about this situation we find ourselves in?"

"Irina," she said. "The young miss is called Irina," she repeated and smiled sweetly across the cabin at the older man. Richard knew he would do anything to have her smile like that at him again, and then he mentally shook himself. What was he thinking? He was a married man in his fifties, he had no business going around acting like a flustered school boy around a young woman, no matter how beautiful!

The Asian man smiled mildly in response. He did not look overly impressed at being the center of Irina's attention. "Miss Irina, then," he said. "I am Mr. Lee. This is Uwe Schmidt."

"*Guten tag*," said Uwe and smiled vacuously.

"Richard Barnaby," said Richard automatically, nodding at his companions.

"Excuse me very much, Richard," said Uwe, looking almost apologetic. "I can get... excited, sometimes."

Richard shrugged. "It's all right," he said. "It's a stressful situation." He glanced around meaningfully. "Hopefully the lift will get going again and this will just be another story we tell our friends and family when we get off this mountain."

Mr. Lee nodded sagely. "It's been five minutes and we still have not started moving again," he said. "It could just be a minor problem and they will get it going again. But, if we are being realistic, it could also mean they didn't notice us getting on and they are shutting down for the night. With this weather, there's little chance anyone will spot us up here. Which means this lift will not start up again until the morning."

"It's going to get cold," Richard said, instinctively huddling in his seat. "If I read that weather report correctly, it'll get too cold, in fact."

"Too cold," agreed Mr. Lee calmly. "Too cold to stay here."

"*Njet*," Irina protested. "What you mean, too cold?"

Mr. Lee thumped the metal siding of the gondola car. There was a hollow sound in response. "See? No heating, no insulation," he said in a voice as if he was discussing the weather. "It will get too cold to stay here overnight. We will freeze to death long before the morning."

Richard swallowed. He was only wearing a thin ski jacket with two layers beneath it. He was already cold, and knew he wasn't dressed for spending the night outdoors in a blizzard. "The lift could still start back up."

Mr. Lee smiled sadly, clearly unconvinced. "True, it could, but I don't like our chances, " he said, turning to Uwe. "Which is why I want Uwe to improve them."

Uwe looked up, clearly startled. "*Was, mich?*" he asked in confusion. "What can I do?"

Mr. Lee smiled mildly again and pointed at Uwe. "Your Nokia," he said. "The mobile phone, right there in your pocket."

*The phone!* Richard thought jubilantly. They could just call down to the lodge to get someone to restart the lift. They were saved!

The study featured up to this point of the story to restrict the sessions in 2 hours. We encourage you to read the full story though ☺

"Ahh," said Uwe, having come to the same happy conclusion. He half-stood to push a hand into his breast pocket, causing Irina's hand to drop from his leg. Richard glanced over to the woman, and caught a curious look on her face. Then it was gone, replaced by an impish curl of her lips as she met his gaze for a single electrifying moment. Again he felt his pulse race, a lump forming in his throat and butterflies swirling in the pit of his stomach, and again he mentally kicked himself for such childish behavior. He was more or less happily married, damn it! This was not the time or the place for flirting with women thirty years his junior.

*Hardly flirting*, he scoffed to himself. *She's toying with me, that's all.*

Meanwhile, Uwe had managed to pull the large black mobile phone out of his breast pocket, and held it up triumphantly like a pike from a sport fishing contest. He beamed down at Irina, who had stepped very close to him, pressing her bosom against him and gazing up at him under long lashes.

*As a matter of fact*, Richard thought clinically as he watched the big stupid grin on the German's ruddy face. *She's toying with us all, isn't she?*

"I don't know about you, but I'm getting cold," said Mr. Lee dryly. "Call the lodge, Uwe, would you please?"

Uwe looked sheepish, and then brought the phone up to his face. Richard held his breath, knowing that those things ran on battery, but was relieved to see Uwe's face light up by an underworldly green glow from the device's little screen. The big man looked decidedly brutish in the fetid light as he punched in numbers on the phone, each press punctuated by a tiny beep that sounded far too loud in the stillness of the cabin. Uwe tapped the big call button on the phone and then raised it to his ear. Glancing at the other occupants, Richard realized everyone was holding their breath now.

Uwe listened, his brow furrowing in confusion. "Nothing," said Uwe. "I hear no phone tone, just... what is that, static?" He brought the phone back to his ear, listening.

Richard once again felt the fangs of fear bite into him, but Mr. Lee looked unperturbed. "Do you have coverage?" he asked calmly.

Uwe looked at the phone display. "Three out of five," he said. "It should work. I just used it earlier today on this lift, do you remember, Mr. Lee?"

"Yes, I do remember," said Mr. Lee. "Maybe try another spot in the cabin, see if you get a better signal somewhere else?"

Uwe nodded and moved away from the bench. He repeated the exercise, and this time he was close enough so that Richard could hear the static from the phone's loudspeaker. He tried a third time from the corner, the gondola car rocking alarmingly as the weight distribution shifted. Richard grabbed the handrail again as vertigo gripped him, and for a moment he was actually grateful that the night was dark and snowy enough that he couldn't see the rocky slope far beneath him. The wind tugged at the car, exacerbating the swing, and he gripped harder.

"Cabin is metal," said Irina. She was still standing in the middle of the gondola, her white snowsuit almost incandescent in the dim light. She didn't seem to mind the wind and was riding the motion like a sailor on a rolling deck. "Metal stop radio waves, yes?"

Mr. Lee looked her way and nodded thoughtfully. "Yes," he agreed. "Metal does interfere with radio waves. But it's not as if we can step off the lift to make a call, is it?"

"No problem," said Uwe, coming over to Richard's side next to the door, his ski boots thumping on the metal. "I try sticking the phone out the window." And without further ado, he pulled down the nearest window and reached out with his hand holding the phone into the free air outside the car.

Richard was still deciding how he felt about this course of events when the wind grabbed the little gondola car once again, this time setting it swinging violently from side to side. Uwe lost his balance and fell towards Richard, who all of a sudden found himself with two hundred pounds of German in his lap, and let out a surprised "ooof" as all the air went out of his lungs. There was a loud bang from the window, followed by a bellow and a string of German curses.

"*Oh mein Gott, das Telefon!*" yelled Uwe from above Richard, frantically scrabbling to his feet and managing to kick Richard in the shin in the process. The blow hit Richard's ski boots, so there was no pain, but a moment later Uwe's elbow connected with his temple, and he saw stars and blacked out.

When he came to, he was slumped back in the seat, and the cabin in front of him had erupted in a chaos of shouting and flailing limbs. Uwe was back on his feet, half leaning out the open window and bellowing into the night, with Mr. Lee behind him holding on to the big German's jacket trying to rein him in, his yellow beanie half covering his eyes. Irina was still standing in the middle of the cabin, impassively looking at the two struggling men with her lips slightly parted. As she noticed his gaze, she looked back at him, biting her lip and nodding meaningfully back at the pair at the window in clear encouragement. Richard got to his feet, still unsteady, his hand coming up to his throbbing temple, and shuffled over as quickly as he could.

"Careful!" he yelled, grabbing Uwe's shoulders and helping Mr. Lee pull the big man safely back into the cabin. Icy tendrils of snow were venting through the window into the cabin and biting at his cheek. "You'll fall if you don't calm down!"

"But the phone!" wailed Uwe, now actually sobbing in great big gulps. "I lost it! I slipped and I lost it! It's gone!!" He made as if to lunge towards the window, but then Irina was there, squeezing up next to him and placing a slender hand on his chest. The fight went out of him instantly, and he sagged back against one of the metal pillars in the middle of the cabin. She was tall, Richard saw, taller than him, but she still had to stand on tiptoe in her white ski boots to put her mouth to Uwe's ear and whisper something.

Richard saw it, and shivered involuntarily. He could imagine himself in Uwe's place, with Irina next to him, pressing her body against his, her soft lips almost touching his hair, and her warm breath fluttering in his ear. He shuddered and had to look away, the wind sweeping in from the window not feeling that cold anymore. Still, he walked up to the window and pulled it shut, hoping to keep the little warmth remaining in the cabin on the inside.

"All right," said Mr. Lee as Irina led Uwe back to their seat, the big man hanging his head in defeat. "The phone is gone. No great loss because it wasn't working anyway." He hiked up the sleeve of his jacket and glanced at a watch. "It's almost five forty and the lift has been stopped for a good half hour. And this storm and the cold is only going to get worse. I think it's time we start thinking about alternatives."

Uwe had buried his head in his big hairy hands, and was muttering in German. Irina was sitting next to him and still pressing her body to him, one of her hands gripping his thigh firmly. She was speaking softly to him under her breath. Richard didn't expect any meaningful contribution from any of them, at least not for the time being.

"Agreed," he said instead, not wanting to leave Mr. Lee hanging. The man seemed to be the only one among them still able to keep a clear head. His own head was swimming with a potent blend of black despair and sheer terror. "But what can we do?"

"Does anyone know we're here?" Mr. Lee said. "Unfortunately, both Herr Uwe and I are here on business, with no friends or family. No one will miss for a couple of days, I'm afraid. What about you, Richard?"

Richard thought about it, a glimmer of hope awakening in his chest. "My wife is in the resort hotel. She will start to wonder where I am if I don't show up." But would she now? Richard wasn't sure. Christa's drinking had been picking up in the last few years, and he had a nagging suspicion she was already a couple of cocktails deep. If he didn't show up in an hour when the live music started, would she even be in a state to notice that he wasn't there, let alone investigate? "At least I hope so," he added. *Please, honey, don't let me down.*

Irina swept them both with her gaze. "Vacation alone," she said curtly and turned back to comforting Uwe. "I come today, I leave Sunday."

"Two days from now," said Mr. Lee grimly. "By that time, this will be over, one way or another." He turned to look at Richard. "It sounds like your wife is our best bet, Richard. When would she expect you?"

"We were supposed to watch the live music in the lodge at seven," Richard said. "But things have been a little... rocky lately. I can't guarantee that she'll actually get someone to come look for me."

Mr. Lee nodded. "It still sounds like a better than average chance she'll raise the alarm," he said. "I suggest we wait until at least seven thirty or so before we start thinking about a plan B."

It wouldn't have been so bad if it wasn't for the cold. Richard was bone tired from not just a whole day on the slopes, but a whole week prior to that, and he was perfectly content to huddle up in his seat and doze. But the frigid cold creeping into the cabin quickly started him shivering uncontrollably, making sleep impossible. Mr. Lee, ever the problem solver, soon got them all to huddle together in the middle of the cabin for warmth, and Richard ended up with Irina's back pressed up against him, Uwe on the other side. Her hair smelled faintly of lilac, and he busied himself for a couple of minutes filling his nostrils with her fresh and clean scent and absorbing the heat radiating from her slender body under the tight snowsuit. When she leaned back against him, unconsciously resting her head against his shoulder, he found his heart racing once again and dared hardly to move for fear of having her change posture. Instead he unobtrusively slipped his arm around her with a confidence he didn't really feel. She didn't object, but instead snuggled a little closer and rested her hands contentedly on his arm draped over her stomach. Uwe was slumped forward with his head in his hands in the seat next to her, breathing heavily, and Irina seemed to have at least temporarily lost interest in him.

Despite his promises that further planning could wait, Mr. Lee didn't seem content to just sit around. Instead he busied himself surveying the gear available to them in the small gondola car. He had quickly found the emergency kit bolted to the underside of the metal bench opposite the accordion doors, and was carefully unpacking the items and lining them up on the floor. He had found a small flashlight in the kit and had rigged it on the bench to shine down on the growing collection. Richard looked over and saw a coil of thin but strong rope, probably a hundred feet if not more, a first aid kit, three liter-sized containers of water, a small jar of white pills, flares, a short-hafted axe, a big survival knife, a stack of Mylar blankets, and a large box of matches. Beyond these, Mr. Lee had gathered their ski poles—four pairs in total—and busied himself for a while with binding them together by their straps into a long chain. Presumably that could be used to hang out the door to scale down to the ground below, even if they measured only perhaps thirty feet in total. Richard thought it looked unsafe and thanked whatever engineer had decided to include an actual rope into the emergency car in the gondola. How far down was the ground anyway?

All the while, the storm outside the gondola raged and worsened, its irritable whine becoming a throaty roar and the buffeting soon turning into a sustained wind that kept the car listing at a five degree angle like a kite streaming in the slipstream behind a racing car. Visibility remained low, with the fluorescent light from the nearby lift pylon flickering under the heavy snowfall sweeping across the mountainside. Worse, the windows were old, letting tendrils of snow to whisper through their patchy seals and fill the interior with a fine mist of ice. Before long, the windows

themselves started to grow big blooms of frost from their collective breath as the temperature in the cabin dropped below freezing.

*It's not going to work*, Richard thought as he felt the cold steal into his body. *I don't think I'll even make it to seven*. At one point the cold was enough that he no longer paid attention to Irina's lithe body leaning against him. And he was starting to feel sleepy, so very sleepy—

"—should be some sign by now," someone was saying from far away. Richard awoke with a start and looked around in confusion. For a moment he didn't know where he was and his mind felt syrupy and slow, as if he was awakening with a hangover from a whole night of drinking. And he was cold! His feet and fingers felt numb, some of them not even seeming to respond.

"I was saying, it's way past seven thirty," someone said again, and Richard looked up in dumb confusion. Mr. Lee was standing over him, looking mildly impatient. "There should be some sign by now if help is coming, but there is none. We need to think about our options."

Richard pushed himself up to sitting, nodding stupidly. Irina was stretching languidly in his lap, seemingly oblivious to the cold and yawning hugely. Her body felt tight like a bowstring against him, strong and muscular, before she relaxed and turned to regard Mr. Lee. Even Uwe was stirring, muttering in German and shaking his head like a bear trying to rid itself of an intrusive fly.

"So, do we climb over to that pylon, or lower ourselves to the ground?" Richard said, trying to shake the cobwebs from his head. "I think I saw a ladder on the pylon, and there's light to shine our way." Neither of those two options sounded very appealing, but intellectually he also knew that they were past half measures. The night was too cold to waste any more time.

"I think the ground is our best bet," Mr. Lee said. "And we don't all have to go. One of us is enough. I'd have the young lady go, on account of being the lightest, but I think it would be better if I went."

Richard raised his eyebrows. "Are you sure?" he said. "I'm a strong skier. I'd be happy to go." *Besides, it'd get me off this damn car and somewhere warm that much faster.*

Mr. Lee shook his head. "You're a large man, Mr. Barnaby", he said. "Not as large as Uwe, but I would much rather have you help him with the rope."

Richard nodded his assent. It made sense, and truth to tell, he wasn't that keen on swinging himself out over a hundred feet of open air above a frigid cliffside.

"Yes, sure," said Uwe, nodding vigorously. "No problem. Richard and I on the rope."

"Good plan," said Irina approvingly, getting to her feet. The loss of her warm body against him was a physical thing, and he scrambled to his feet as well to cover it up. "Tell me how I can help."

"All right, let's do it," said Mr. Lee. He was holding the big coil of rope in his hands. "This rope is plenty strong enough, and there's 150 feet of it. I'd prefer if we tied a harness so that you three can lower me instead of having me lower myself. It's just too cold for me to trust my grip in these conditions."

They quickly got to work, Richard tying a harness and Uwe treading the rope around the sturdy center pillar and bracing it against one of the metal benches. Irina helped Mr. Lee open the door, exposing the interior of the car to the howling wind, and secured it in the open position. The little Asian man then picked up his skis from the nearby rack, and, holding them straight out the open door, let them fall to the ground below. There was a crash, but Richard couldn't tell if the skis had broken or not. The remaining skis quickly followed suit. Hopefully at least one had survived the fall.

Mr. Lee wriggled into the harness and tested it carefully. Satisfied with the fit, he stepped up to the open door, turned, and gave them his mild smile. "Wish me luck," he said. "I should be back in a half hour, and an hour at the most. Hang in there and keep moving."

"Good luck, Mr. Lee," said Uwe solemnly.

Richard shook the man's hand. Then Mr. Lee sat down on the floor and scooted up to the doorway. Uwe and Richard collected the slack, and Mr. Lee turned on his stomach and let his feet and legs dangle out the open door. He looked up at Richard and Uwe, and then slid carefully backwards into the void. The two men braced themselves against metal pillars in the cabin and easily took the man's weight. Uwe grunted, and together they started to carefully pay out the rope, a foot at a time, to lower Mr. Lee to the ground far below the gondola car.

What happened next was so unexpected that Richard at first thought he was dreaming. Suddenly Irina swept past him, fluttering dark locks and a smell of lilacs in her wake, and walked up next to Uwe's hulking form beside the open door. She put her hand on his chest again, instantly making the big man freeze, and stood on her tiptoes to whisper something in his ear. Uwe momentarily tilted his head as if in confusion, but then Irina was stepping back again and now Uwe was turning abruptly towards him, and Richard barely had time to register the ham-like fist coming up towards him before it connected.

He didn't lose consciousness this time, but the crash against the metal bulkhead was enough to drive the air out of his lungs and leave him gasping for breath on the floor of the cabin. When he was finally able to prop himself up on an elbow, it was just in time for him to see Uwe straightening up from the metal bench with the rope in one hand, clearly having undone the knot securing the rope to the car. Without a moment's hesitation, the big German let go, and the rope quickly snaked out the open door and disappeared. There was no sound. If the little man at the end of that rope went to his death screaming, the storm's roar was loud enough to hide it from Richard's ears.

Richard laboriously got up to a sitting position, sliding up next to the wall behind him as Uwe turned to look at him with murderous rage in his dumb little eyes. Richard's heart was thumping harder than it had ever done before, and for a moment he thought he'd suffer a heart attack

right there on the spot. *But no*, he thought with a surprising sense of detachment. *That's not what's going to kill me. Uwe is what's going to kill me.*

"Now him, Uwe," Irina said calmly, as if to echo his thoughts. She was leaning against the metal railing next to the open door in a posture of relaxed leisure, long legs crossed nonchalantly and avid eyes watching them both. Her voice had taken on a throaty purr that somehow seemed to dig its claws into Richard's lower abdomen. "And then you can have me, my love. Right here on the floor."

Uwe grunted with animalistic lust, rising from his half crouch to his full height. His arms hung down like that of a great ape, the big hands grasping at empty air. Richard felt the fear dig its fangs even deeper into him, and he pressed himself against the metal, as if he could somehow tunnel through it and—

His hand fell on a tubular object on the floor next to him. He knew it was the axe even before he dared to glance down. Mr. Lee had even helpfully unsheathed it from its protective cover, and he gripped it in his gloved hand..

Uwe charged.

The cabin wasn't big, and Richard barely had enough time to swing the axe. If Uwe had gotten his hands on Richard, it would have been all over, all his strength sapped in a moment by the chokehold and the big man's massive shoulders protecting him from any glancing blow he could have struck at that point. Richard barely had enough time, but only barely.

The axe sliced into Uwe's face at the apex of its upward arc, splitting lips, splintering teeth, and shearing off the man's lower jaw. Richard felt warm blood spray his face, and instinctively closed his eyes and turned his head. There was a guttural roar, but no huge hands came grasping for his throat, and after a moment Richard began to scramble to his feet and look up.

Uwe was stumbling backwards in the confined space, both hands feeling in confusion for his missing jaw. The entire front of his snowsuit was covered in a sheet of blue-black blood. All the while the man was making that low guttural sound, like an animal in mortal pain. An animal with no lower jaw and thus no longer able to speak. As if sensing the void behind him, the big German froze in the doorway and let his hands fall powerlessly to his side.

That was when Irina stepped up to Uwe, and with the precision of a surgeon, calmly slit his throat from ear to ear with the survival knife from the emergency kit. The big man grabbed feebly at his throat, dark heartblood spilling out like hot tar between his fingers, eyes swiveling from Richard to fixate on Irina's face in a look of comic confusion. She smirked, head tilting back and lips parting as she leaned in and kissed him passionately on his ruined half-mouth, unmindful of the blood. Then she stepped back, delicately placed a ski boot against his midsection, and pushed. The man swayed precariously for a moment before toppling backwards out the open door without a sound. Irina turned on her heel with catlike grace and fixed Richard with her purple eyes. They looked as if they were almost lit from within.

"So, it turned out to be you in the end," she said conversationally, all traces of Russian accent gone from her voice. Now her speech was cultured and with a slight British accent. "I wouldn't have thought so at first, but who am I to judge?"

She shrugged eloquently, the gory survival knife still held in one exquisite hand. There was a Rorschach spatter of blood across her face, crimson against white, but as his eyes met hers he thought he had never seen anything so beautiful in his whole life. He felt his own arousal rising, his pulse pounding in his ears.

"Well, I guess you'll have to do," she gasped quietly, almost to herself, and let her hand drop, the knife clattering to the floor.

There was desire in her eyes now. Her tongue came out, pink tip darting up and tasting the blood with something like satisfaction, and then all of a sudden she had covered the distance between them in two long strides, her face filling his vision. He dropped the bloody axe and fell back on the hard metal bench behind him and now she was straddling him, her long legs, so long, gripping him firmly, and her arms came up over her head, and then her jacket was off and all he could see were her big purple eyes and he knew she was naked and oh how he wanted to look but her eyes were just so big and she was bending down for a kiss and oh my god her eyes her eyes her eyes—

Valle d'Aosta, Italy - Dec 14, 1992 (ANSA) - Italian authorities today released the identity of the three tourists who tragically died in a ski lift accident in the Pila ski resort in Italy's famous Valle d'Aosta ski area over the weekend. One of the three was American businessman Richard Barnaby, who was visiting the area on vacation with his wife. The other two, both men, were of German and Singaporean nationality. The trio were stranded in a gondola car more than 100 feet above the ground on the evening of Friday, December 11 when the lift shut down halfway through their passage up the mountain. Resort management claims that typical safety protocols failed, and the low visibility due to an incoming blizzard prevented personnel from spotting the occupants of the gondola car. After what appears to be a couple of hours of hesitation, the trio performed a daring escape attempt using an emergency rope, but weather conditions were too poor, causing two of the three to fall to their deaths. Mr. Barnaby was found as the sole remaining occupant in the gondola car, having frozen to death sometime during the night. Richard Barnaby is survived by his wife Christa, who was questioned by...
