# Supplementary material for: DramatVis Personae: Visual Text Analytics for Identifying Social Biases in Creative Writing
Source: arXiv:2209.00320 source file (2022-09-01)
Supplement: Supplementary file 2 [file The-prisoners.pdf]

| Character | Gender     | Race  | Age         |
|-----------|------------|-------|-------------|
| Jackson   | Male       | Black | Young       |
| Eric      | Male       | White | Middle-aged |
| Jane      | Female     | Black | Middle-aged |
| Monica    | Female     | Black | Middle-aged |
| Chang     | Non-binary | Asian | Old         |

The bars of the prison seemed indestructible and no sound escaped the deafening walls.

The hallway outside appeared deserted and a suffocating aura loomed all over. Jackson banged his fists frustratingly against the prison bars and gritted his teeth in irritation.

“Why waste your energy, young man? When you know that there is no use of your youthful strength against those bars of metal?” Chang demanded with a naughty smile on his aging face.

Jackson turned around and slid down with his back against the bars in helplessness. Eric sat in a corner, playing with his Swiss knife that he had managed to sneak into the prison. The atrocious tattoo burnt against his face that was shaped in the form of a cobra made him look even more intimidating.

He looked at Jackson and inquired loudly with a smirk curling across his pierced lips.

“Yo, genius! How did an innocent punk like you land up in here?”

Jackson, however, was filled with intense agony and frustration to even gather the inner will to reply and merely sat there hopelessly.

“Hey dude, I’m asking you something!” Eric shouted.

“Shut your mouth, Eric! The kid looks disturbed, leave him alone!” Jane snapped as she lay in the opposite corner taking a sip from her tiny bottle of beer. Eric glared at her with a dirty look on his face but managed to keep his temper under control.

Monica, on the other hand, lay with her arm on her forehead on the ground and merely stared at the blank white ceiling.

Eric spat on the ground and turning his attention towards Chang, he demanded,

"You! Asian guy! What could a person like you have possibly done to land up in this shithole?"

Chang began to chuckle insanely and replied,

"Well, I was sent here for killing my insufferably annoying younger brother,"

"What! You don't look like a killer in any way, old man!" Eric laughed coldly, revealing his dirty yellow teeth.

"Well, young man. You don't need to use violence to remove a person out of this world. All I had to do was mix a few drops of rat poison in his bottle of liquor and whoosh... he was gone,"

"But why on earth would you do that?" Jane asked in a serene tone.

"Missy, the outside world is a hell for eunuchs like me. Even our own family members despise us to the limit, and my brother would have anyway killed me if I hadn't done it myself,"

"What do you mean?" she demanded in confusion.

"He was hatching a plan to have me thrown into the sea while I slept, but I became aware of his plan and decided to send up, before he had the chance to send me,"

Eric sniggered humorously and flipped the Swiss knife back into his pocket.

"So, how long have been here, old man?"

"Twenty-years, this may," he answered with a brief sigh of disappointment.

"What about you? How did a charmingly beautiful maiden like you find a path to this horrible place?" Chang asked Jane who looked quite cold at the question.

"For stabbing my drunkard father in the back, who would hit my mum every night after returning home from gambling and losing all of his money," her tone seemed cold, yet very emotional.

"I'm sorry, girl," Chang expressed regretfully while Eric simply maintained his despicably bitter expression.

After a moment of deafening silence, a series of footsteps were heard from outside which immediately diverted their attention from their sickening tragedies.

An officer approached their cell and slid four plastic trays of stale food towards them.

"Eat! You filthy maggots! Remember! You got work tomorrow!" he barked at them, but the moment he turned his back against them, Jackson jumped onto his feet and wrapped his arm across his throat while he began to choke silently. The officer struggled to free himself,

but in vain, as Jackson's grip was extremely firm. His face was expressionless as he choked the man. After a long struggle, the officer stopped moving and lay motionless, with his eyes staring in space soullessly. Jackson shoved his hand in his pocket and removed the key. He released the officer, who fell to the ground, and then began to work on the prison lock which opened quickly and the bars slid aside.

"Way to go, pal!" Eric cheered in exhilaration while the rest of them rushed out of the prison quickly.

The five moved cautiously across the dungeon and remained alert.

They heard a few more steps descending from the stairs and the five of them moved aside with their backs against the wall. Eric opened his mouth to speak but Jackson gestured him to remain silent with a stone cold look. Another tall officer marched down the stairs and before they could reach their cell, Jackson grabbed the officer and clamping his hand on his mouth, he delivered a series of gut-wrenching blows on his lower back and twisted his neck, while the rest of them stared at him in shock. Leaving the dead officer on the ground, they resumed moving but Chang halted them abruptly.

"Wait, I know a place from where we can escape without being seen!" He blurted and they all followed the slow old man.

Chang took them towards the opposite end of the dungeon where a large metallic lid appeared on the ground.

"Jackpot!" Eric shouted while Monica threw him an irritated look and his smile vanished under her piercing glare.

Jackson moved the lid aside briskly and a pitch-black tunnel emerged. Monica looked down in shock and moved back.

"I am not jumping in that dirty hole! I'd rather go back and lie in the prison!" she exclaimed in a disgusted voice.

"Are you out of your mind?" Jane demanded, widening her eyeballs.

Without wasting another second, Jackson and Eric jumped down the hole. Meanwhile, they heard a few more footsteps across the dungeon.

"Let's go!" Jane shouted and finally, Monica was ready to jump alongside Jane. Chang, on the other hand, merely watched them as they began to jump through the massive hole.

Eventually, Jane gestured him to come, but he merely smiled and did not move.

“What’s wrong with your?” she yelled, but the old eunuch continued to smile and moved back. In the interim, the police officers arrived and saw them escaping.

“Hey you! Stop right there!” they roared and opened fire. As the spray of bullets tore through the old Asian’s chest, a trickle of tear flowed across Jane’s cheek as she jumped down through the hole. The four of them landed in an enormous tunnel which horribly smelled of dead rats and polluted water.

“Where is that old man?” Eric inquired and Jane nodded her head coldly as they rushed through the tunnel.

In the meantime, the officers jumped into the tunnel as well and turned on their torches to look for the prisoners.

But, before the officers could go much further, there was a splash of water from below as Jackson pounced on them from behind. He caught their shins and threw them onto the watery floor. One of the officers tried to shoot but he was knocked out cold with the black man’s punch who then twisted his neck. The other officer tried to shoot but Jackson pushed his face into the water and held there firmly. After writhing like a fish, the officer remained still.

“Dammit, who the hell is this guy?” Monica expressed in shock while Jane and Eric stared at him with their jaws dropped.

“Couldn’t you stop him from killing them outright?!” Jane whispered to Eric who looked disturbed.

“I am a small time thief! I don’t get involved in fights and murders!” he said loudly.

After putting an end to the officers, Jackson took their handguns and gestured them to follow him. The four prisoners ran across the spooky tunnel and arrived at a dead end with a massive lid stuck to the wall.

Jackson and Eric moved it aside together and the sparkling rays of the sun struck their faces. They looked down and noticed a huge lake lying nearly a hundred metres below.

“We need to jump!” Jackson spoke and the rest looked mildly amazed. But the words had barely escaped his lips when they heard few officers running from the other end.

“Let’s jump, quickly!” Eric said, but Jackson shockingly aimed the handgun at him.

“Sorry pal, but there is only one ticket to freedom here,” he declared as an evil smirk spread across his lips.

“Dude! Are you crazy?” Monica demanded.

“Well, a man who has committed five murders and three rapes is crazy, lady!” he replied, leaving them thunderstruck.

Saying that he waited till the officers were nearby and dived below into the lake...leaving the other four into the clutches of law.
