# Supplementary material for: DramatVis Personae: Visual Text Analytics for Identifying Social Biases in Creative Writing
Source: arXiv:2209.00320 source file (2022-09-01)
Supplement: Supplementary file 3 [file study_questions.pdf]

This file includes the questions along with the multiple choices designed for the user study. The correct answers are presented in bold. Two authors of this research separately and manually analyzed the stories to get the correct answers and verified them by discussing with each other. The correct answers were also validated by the writers of the stories. The questions appeared in random order to the participants.

## Questions for A Kiss of Ice

1. Which of the following characters has the most presence in the story?
  - a. **Irina (The Woman)**
  - b. Uwe (The Bearded Man)
  - c. Christa Barnaby
  - d. Mr. Lee (The Asian Man)
2. Which of the following characters has the least presence in the story?
  - a. Richard Barnaby
  - b. Irina (The Woman)
  - c. Uwe (The Bearded Man)
  - d. **Mr. Lee (The Asian Man)**
3. Which of the following social identities has the least presence in the story?
  - a. Young
  - b. Female
  - c. German
  - d. Russian
  - e. **Old**
4. Which of the following two characters have the most interactions (having conversations, or participating at a scene together) with each other in the story?
  - a. Richard Barnaby and Uwe (The Bearded Man)
  - b. **Richard Barnaby and Irina (The Woman)**
  - c. Richard Barnaby and Christa Barnaby
  - d. Irina (The Woman) and Mr. Lee (The Asian Man)
  - e. Irina (The Woman) and Uwe (The Bearded Man)
5. Which of the following two characters have the least interactions (having conversations, or participating at a scene together) with each other in the story?
  - a. Richard Barnaby and Uwe (The Bearded Man)
  - b. Richard Barnaby and Irina (The Woman)
  - c. Richard Barnaby and Christa Barnaby
  - d. **Irina (The Woman) and Mr. Lee (The Asian Man)**
  - e. Irina (The Woman) and Uwe (The Bearded Man)
6. Which of the following characters was portrayed as aggressive in the story?
  - a. Richard Barnaby
  - b. **Uwe (The Bearded Man)**
  - c. Irina (The Woman)
  - d. Christa Barnaby

- d. Mr. Lee (The Asian Man)
- 7. How would you categorize how Female characters were portrayed in the story?
  - a. Funny and Sarcastic
  - b. Aggressive and Powerful
  - c. **Passive, Beautiful, and Sulky**
  - d. Active and Glorified

## Questions for The Prisoners

1. Which of the following characters has the most presence in the story?
  - a. **Jackson**
  - b. Eric
  - c. Chang
  - d. Jane
  - e. Monica
2. Which of the following characters has the least presence in the story?
  - a. Jackson
  - b. Eric
  - c. Chang
  - d. Jane
  - e. **Monica**
3. Which of the following social identities has the least presence in the story?
  - a. Young Male Black
  - b. Middle-aged Female Black
  - c. Old Non-binary Asian
  - d. **Middle-aged Male White**
4. Which of the following social identities has the second least presence in the story?
  - a. Male Black
  - b. Female Black
  - c. **Non-binary Asian**
  - d. Male White
5. Which of the following two characters have the most interactions (having conversations, or participating at a scene together) with each other in the story?
  - a. Jackson and Chang
  - b. **Jackson and Eric**
  - c. Jackson and Jane
  - d. Jane and Chang
  - e. Eric and Monica
6. Which character was portrayed as rude and bitter in the story?
  - a. Jackson
  - b. **Eric**
  - c. Chang
  - d. Jane

e. Monica

7. How would you categorize how Female characters were portrayed in the story?

a. Aggressive and Powerful

b. **Beautiful, distressed, and Emotional**

c. Funny and Sarcastic

d. Active and Glorified
